# Supplementary material for: Behavior Cloning for Mini Autonomous Car Path Following
Source: arXiv:2410.07209 source file (2024-09-25)
Supplement: Supplementary file 1 [file 0_1_supplementary_material.tex]

\section*{Supplementary Material}\label{supplementary_material}

Video of the experiments available at: \texttt{\url{https://youtu.be/PqTDzsKjA9c}}. 
Released code at: \texttt{\url{https://github.com/ricardoGrando/DoCRL}}.
